# Supplementary material for: Fast image reverse filters through fixed point and gradient descent acceleration
Source: arXiv:2206.10124 source file (2022-06-21)
Supplement: Supplementary file 1 [file supplementary_material.tex]

\newpage
\setcounter{section}{0}
\huge{\textbf{Supplementary material}}

\section{Adaptive Manifolds for Real-Time High-Dimensional Filtering}

\begin{figure}[h!]
    \centering
    \begin{subfigure}{0.24\linewidth}
        \includegraphics[trim=0 0 0 0, clip,width=\linewidth]{New_images/AMF/PSNR_T_AFP_AMF.eps}
        \caption{T-Method}
        \label{fig:T_APF_PSNR2}
    \end{subfigure}
    \begin{subfigure}{0.24\linewidth}
        \includegraphics[trim=0 0 0 0, clip,width=\linewidth]{New_images/AMF/PSNR_TDA_AFP_AMF.eps}
        \caption{TDA-Method}
        \label{fig:TDA_AFP_PSNR2}
    \end{subfigure}
        \begin{subfigure}{0.24\linewidth}
        \includegraphics[trim=0 0 0 0, clip,width=\linewidth]{New_images/AMF/PSNR_P_AFP_AMF.eps}
        \caption{P-Method}
        \label{fig:P_AFP_PSNR2}
    \end{subfigure}
            \begin{subfigure}{0.24\linewidth}
        \includegraphics[trim=0 0 0 0, clip,width=\linewidth]{New_images/AMF/PSNR_P2_AFP_AMF.eps}
        \caption{New P-Method}
        \label{fig:P2_AFP_PSNR2}
    \end{subfigure}

    \caption{Reversing an AMF filter with different reverse filtering methods and accelerated fixed point iteration.}
    \label{fig:AFP_PSNR2}
\end{figure}

\begin{figure}[h!]
    \centering
    \begin{subfigure}{0.24\linewidth}
        \includegraphics[trim=0 0 0 0, clip,width=\linewidth]{New_images/AMF/PSNR_T_AGD_AMF.eps}
        \caption{T-Method}
        \label{fig:T_AGD_PSNR2}
    \end{subfigure}
    \begin{subfigure}{0.24\linewidth}
        \includegraphics[trim=0 0 0 0, clip,width=\linewidth]{New_images/AMF/PSNR_TDA_AGD_AMF.eps}
        \caption{TDA-Method}
        \label{fig:T_AGD_PSNR2}
    \end{subfigure}
        \begin{subfigure}{0.24\linewidth}
        \includegraphics[trim=0 0 0 0, clip,width=\linewidth]{New_images/AMF/PSNR_P_AGD_AMF.eps}
        \caption{P-Method}
        \label{fig:T_AGD_PSNR2}
    \end{subfigure}
            \begin{subfigure}{0.24\linewidth}
        \includegraphics[trim=0 0 0 0, clip,width=\linewidth]{New_images/AMF/PSNR_P2_AGD_AMF.eps}
        \caption{p-Method}
        \label{fig:T_AGD_PSNR2}
    \end{subfigure}

    \caption{Reversing an AMF with different reverse filtering methods and accelerated gradient descent.}
    \label{fig:AGD_PSNR2}
\end{figure}    

\begin{figure}[h!]
    \centering
    \begin{subfigure}{0.24\linewidth}
        \includegraphics[trim=0 3cm 0 0, clip,width=\linewidth]{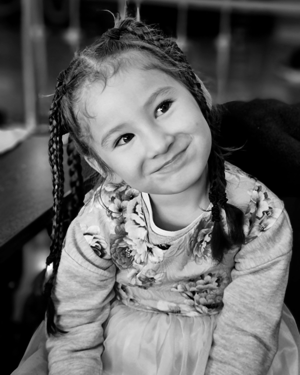}
        \caption{Ground Truth}
    \end{subfigure}
        \begin{subfigure}{0.24\linewidth}
        \includegraphics[trim=0 3cm 0 0, clip,width=\linewidth]{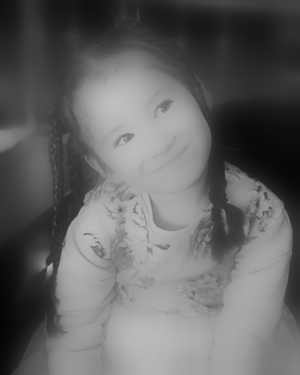}
        \caption{Input image}
    \end{subfigure}
        \begin{subfigure}{0.24\linewidth}
        \includegraphics[trim=0 3cm 0 0, clip,width=\linewidth]{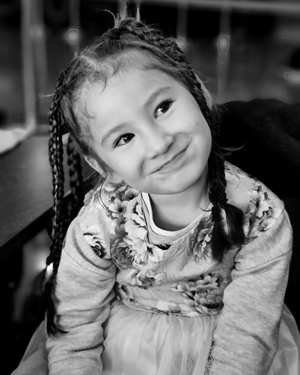}
        \caption{T-method}
    \end{subfigure}
        \begin{subfigure}{0.24\linewidth}
        \includegraphics[trim=0 3cm 0 0, clip,width=\linewidth]{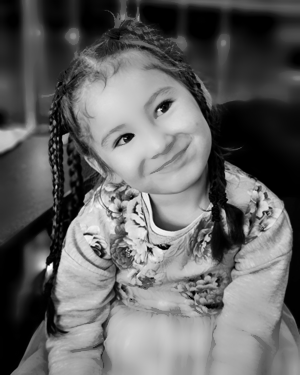}
        \caption{TDA-method}
    \end{subfigure}
        \begin{subfigure}{0.24\linewidth}
        \includegraphics[trim=0 3cm 0 0, clip,width=\linewidth]{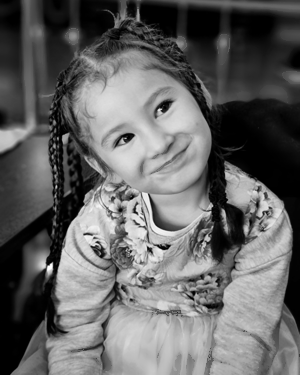}
        \caption{P-method}
    \end{subfigure}
            \begin{subfigure}{0.24\linewidth}
        \includegraphics[trim=0 3cm 0 0, clip,width=\linewidth]{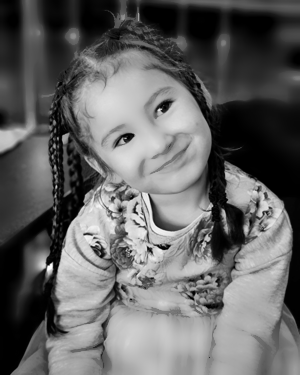}
        \caption{p-method}
    \end{subfigure}
   \begin{subfigure}{0.24\linewidth}
        \includegraphics[trim=0 3cm 0 0, clip,width=\linewidth]{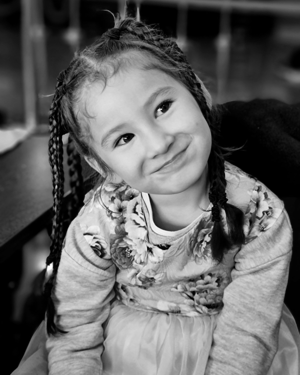}
        \caption{T+AFP}
    \end{subfigure}
     \begin{subfigure}{0.24\linewidth}
        \includegraphics[trim=0 3cm 0 0, clip,width=\linewidth]{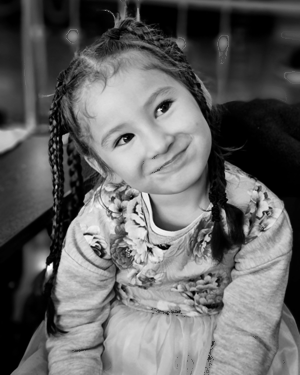}
        \caption{T+AGD}
    \end{subfigure}
    
    \caption{Reversing an AMF filter with different reverse filtering methods. a) Ground truth image, b) Input blurred image, c) d) e) f) results using the classic T, TDA, P and p methods respectively without modification. g) Best result applying AFP which was achieved by the T+AA method, h) best result applying AGD achieved by T+SGDR.}
    \label{fig:GF_visual}
\end{figure}
